# Supplementary material for: Kinetic energy fluctuation-driven locomotor transitions on potential energy landscapes of beam obstacle traversal and self-righting
Source: arXiv:2304.04603 source file (2023-04-10)
Supplement: Supplementary file 1 [file ch6_appendix.tex]

\chapter{Appendix}
\label{chap:appendix}

\footnotetext{Parts of this appendix have been published in the paper “Locomotor transitions in the potential energy landscape-dominated regime” by Ratan Othayoth, Qihan Xuan, Yaqing Wang, and Chen Li in the journal \textit{Proceedings of the Royal Society B: Biological Sciences} \citep{othayoth2021b}}

\section{General steps to create and use potential energy landscapes}

Here I summarize general steps to calculate and use them (also see Figure \ref{fig:a1_pel_steps}).

\begin{enumerate}

\item Create a simplified physics model of the interaction with which system potential energy can be calculated as a function of relevant system degrees of freedom. In our studies, we focused on first understanding coarse-grained transitions between modes that differ significantly in how the body moves. Thus, to create the simplest potential energy landscape with minimal degrees of freedom, we approximated the animal or robot as a rigid body and neglected the legs. We used an ellipsoidal body shape resembling the animal body, except in the pillar study where different body shapes were studied. In addition, we assumed that the body does not penetrate the obstacle or ground and its lowest point is always in contact with the ground. See Sections S3-S7 for other assumptions specific to each model system. Finer-grained transitions between more nuanced modes that involve body bending and leg motion can, in principle, be studied using higher-dimensional potential energy landscapes, although more challenging—see reviews of energy landscape modeling of protein folding (e.g., \cite{wales2003a}).
\item	Quantify system potential energy as a function of system degrees of freedom and physical/geometrical properties. For gap, bump, pillar, and self-righting interaction where body parts are assumed rigid and terrain elements are rigid and fixed, system potential energy is the body gravitational potential energy ($E = mgz_{com}$, where $m$ is the body mass, $g$ is gravitational acceleration, and $z_{com}$ is body center of mass height). For beam interaction, in addition to body gravitational potential energy, beam gravitational energy and elastic potential energy also contribute to system potential energy.
\item	Measure relevant physical/geometrical properties (such as beam stiffness, body mass/geometry) required to calculate system potential energy.
\item	Choose the few system state degrees of freedom over which the potential energy landscape is to be constructed. Often degrees of freedom that represent self-propulsion (e.g., body forward position relative to obstacles, wing opening angle in ground self-righting) and those that change substantially in response to terrain interaction (e.g., body pitch, roll, yaw) are chosen. Because a high-dimensional landscape over a large number of degrees of freedom is more challenging to understand three degrees of freedom can be chosen first to visualize the landscape more easily, as a potential energy map over two degrees of freedom which further evolves over the third degree of freedom. See Section S8 for visualizing the potential energy landscape over all three chosen degrees of freedom. We note that constructing the landscape over only three degrees of freedom is a compromise to simplify analysis and already provide substantial insight into experimental observations. More rigorous analysis of high-dimension landscape over all relevant degrees of freedom and comparison to experimental observations may reveal additional insight in the future.
\item	 Calculate the potential energy landscape over the first two chosen degrees of freedom while keeping the third (and other) degrees of freedom constant. Varying both these degrees of freedom in small increments over the desired range and calculating the potential energy at each point of the grid in this 2-D parameter space.
\item	Construct the evolving potential energy landscape by repeating step 5 while varying the third (and remaining) degrees of freedom, either using an experimentally measured trajectory or prescribing a trajectory.
\item	Visualize system state trajectory on the landscape, by projecting the measured or prescribed values of the first two chosen degrees of freedom on the evolving potential energy landscape. Use only the end points of the trajectory, which represent the current state, to show the actual potential energy of the system. Use the rest of the visualized trajectory to show how measurements of the first two chosen degrees of freedom evolve on the landscape. Because the potential energy landscape evolves as the third degree of freedom changes and can occlude the trajectory, project the trajectory onto the landscape surface for visualization.
\item	Find local minima and identify basins of the landscape. For landscapes with simple shapes, basins can be identified from visual inspection. A more rigorous method is to use graph search algorithms \citep{cormen2009a} to first find the saddle points on the landscape and then identify the basins separated by them.
\item	Determine the potential energy barrier for transitioning from one basin to another, which occurs at the saddle separating the basins. For landscapes with relatively simple shapes, this can be done in several steps. First, consider imaginary straight paths on the landscape away from one basin minimum towards the direction of another basin. Then, along each imaginary straight path, obtain a cross section of the landscape and measure the barrier along this cross section as the maximal increase in potential energy to escape from the basin along the straight path. Repeat this step to calculate potential barriers for transitioning along all possible directions to transition to the other basin. The lowest barrier among all of them is the barrier to transition from this basin to the other. See \cite{othayoth2020a} for detailed steps. A more rigorous method is to calculate the potential energy increase from the basin minimum to the saddle point separating it from another basin using  graph search algorithms \citep{cormen2009a}.
\item	Repeat steps 7-9 to measure system potential energy and potential energy barrier for transition from one basin to another as the third degree of freedom is varied. 
\item	Additional metrics, such as potential energy of basin minima, kinetic energy fluctuation, direction of system state velocity on the landscape, and energy landscape gradients, may be measured. Together, these help understand system behavior and principles of transitions across landscape basins.
 
\end{enumerate}

Below, we briefly summarize specifics of calculating the potential energy landscape of each model system. See respective original studies (Gart and Li, 2018; Gart et al., 2018; Han et al., 2021; Othayoth and Li, 2021; Othayoth et al., 2020; Wang et al., 2021b) for more detail, except the landscape of gap interaction which is first presented here. Note that here we renamed some modes from those in the original studies to better distinguish modes across different model systems. See (Othayoth et al., 2021a) for data, code and interactive plots of potential energy landscapes.

\begin{figure}
    \centering
    \includegraphics[width=1.0\linewidth]{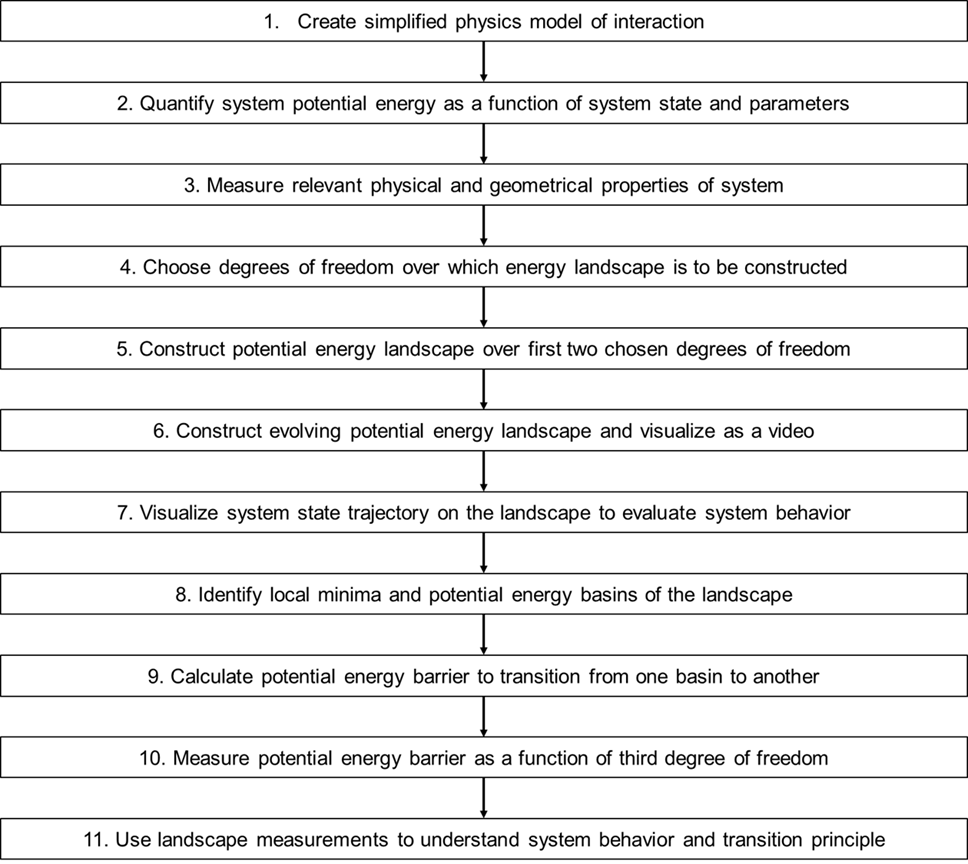}
    \caption[General steps to calculate and use potential energy landscape of locomotor-terrain interaction.]
    {General steps to calculate and use potential energy landscape of locomotor-terrain interaction.}
    \label{fig:a1_pel_steps}
\end{figure}

\clearpage

\section{Potential energy landscape of gap interaction}
A previous study of dynamic traversal of large gap obstacles, we focused on understanding and predicting successful traversal dynamics by creating a template model of gap crossing \citep{gart2018b}. However, a potential energy landscape approach can also provide insight into the emergence of both successful crossing and falling and strategies to make the desired transition. Here I include my a very brief contribution towards developing potential energy landscapes of gap obstacles, which was published as a supplementary of \cite{othayoth2021b} 

We calculated the potential energy landscape of body-gap interaction over the body pitch-yaw space as the body moves forward (figures S2). Throughout traversal, we constrained the body to maintain contact with the ground or the bottom of the gap and not penetrate the vertical sides of the gap. Although the body often lost contact with ground momentarily during crossing in animal and robot experiments, this constraint was required to use the potential energy landscape to model the fall mode. For a given body forward position x, we varied body pitch and yaw over [$-90\degree, 90\degree$] and calculated body potential energy from this constraint. Note that positive pitch corresponds to the body pitching head down.

Before encountering the gap, the body moves forward on level ground (figure S2a, i). In this case, potential energy depends only on body pitch and not on body yaw. The potential energy landscape has a global minimum valley along zero body pitch (figure S2c, i). As the body moves over the gap, pitching downwards lowers the center of mass and reduces potential energy (figure S2a, ii’). As a result, the initial global minimum valley shifts in the positive pitch direction (positive pitch is pitching head down), and a new fall basin develops around it (figure S2c, ii). In the fall basin, potential energy also depends on body yaw because, beyond a certain yaw, the body must pitch up to not penetrate the gap’s vertical sides. Similarly, as the body continues to move forward in the gap, it must pitch down further to not penetrate the far vertical side of the gap. Alternatively, it can pitch up until its bottom contacts the farther edge of the gap. Because increasing or decreasing pitch increases potential energy, a cross basin also emerges, centered around the pitched-up state (figure S2c, iii).

Approaching the gap more slowly and/or with a lower body pitch and/or higher body yaw magnitude decreases the system’s initial kinetic and/or potential energy and increases its probability of being trapped in the fall basin, resulting in the body falling into the gap (figure S2a ii’). After falling, the body can turn sideways (for a sufficiently wide gap) and move within the gap (figure S2a ii’-iii’, c ii’-iii’). By contrast, approaching the gap head-on (with less body yaw), more rapidly, and/or with a higher body pitch (figure S2a ii, c ii) increases the system’s initial kinetic and/or potential energy and increases its probability of overcoming the potential energy barrier to reach the cross basin (figure S2a iii, c iii), resulting in the body crossing the gap. These modeling insights are consistent with those from the dynamical template \citep{gart2018b}.

% \begin{figure}
%     \centering
%     \includegraphics{}
%     \caption{Caption}
%     \label{fig:my_label}
% \end{figure}
